# Supplementary material for: In-Context Learning of Energy Functions
Source: arXiv:2406.12785 source file (2024-06-18)
Supplement: Supplementary file 1 [file 99_appendix.tex]

\appendix
\onecolumn
